# Supplementary material for: Superconductivity in three-dimensional interacting doped topological insulators
Source: arXiv:2407.08736 ancillary file (2024-11-04)
Supplement: Supplementary file 1 [file supplementary.pdf]

# Supplemental Material:
# Superconductivity in three-dimensional interacting doped topological insulators

András L. Szabó[1] and Bitan Roy[2]

[1] *Institute for Theoretical Physics, ETH Zurich, 8093 Zurich, Switzerland*

[2] *Department of Physics, Lehigh University, Bethlehem, Pennsylvania, 18015, USA*

(Dated: July 11, 2024)

The Supplemental Material contains the Fierz reduction of local quartic interaction terms [Sec. I] and provides the explicit form of the renormalization group flow equations [Sec. II and Figs. 1 and 2]. We also display the phase diagrams for individual interaction channels [Sec. III and Figs. 3 and 4].

## I. FIERZ REDUCTION OF QUARTIC TERMS

The interacting Lagrangian in Eq. (2) of the main text contains eight symmetry-allowed local four-fermion terms. However, the number of linearly independent four-fermion terms can be reduced by invoking the Fierz identity [1], given by

$$(\Psi^\dagger M \Psi)(\Psi^\dagger N \Psi) = -\frac{1}{D^2}\mathrm{Tr}(M\Gamma^a N \Gamma^b)(\Psi^\dagger \Gamma^b \Psi)(\Psi^\dagger \Gamma^a \Psi), \tag{1}$$

where $M$ and $N$ are $D$-dimensional Hermitian matrices, with $D = 4$ in our model, and $\Gamma^a$ span a basis in the space of such matrices. We start by arranging the quartic terms in an array according to

$$\mathbf{X}^\top = \Big[(\Psi^\dagger\Gamma_{00}\Psi)^2, (\Psi^\dagger\Gamma_{10}\Psi)^2, (\Psi^\dagger\Gamma_{20}\Psi)^2, (\Psi^\dagger\Gamma_{30}\Psi)^2, \sum_{s=1}^{3}(\Psi^\dagger\Gamma_{0s}\Psi)^2, \sum_{s=1}^{3}(\Psi^\dagger\Gamma_{1s}\Psi)^2, \sum_{s=1}^{3}(\Psi^\dagger\Gamma_{2s}\Psi)^2, \sum_{s=1}^{3}(\Psi^\dagger\Gamma_{3s}\Psi)^2\Big],$$

and use Eq. (1) to write each term as a linear combination of the others. These linear relations can be summed up as $F\mathbf{X} = 0$, with the Fierz matrix

$$F = \frac{1}{4}\begin{pmatrix} 5 & 1 & 1 & 1 & 1 & 1 & 1 & 1 \\ 1 & 5 & -1 & -1 & 1 & 1 & -1 & -1 \\ 1 & -1 & 5 & -1 & 1 & -1 & 1 & -1 \\ 1 & -1 & -1 & 5 & 1 & -1 & -1 & 1 \\ 3 & 3 & 3 & 3 & 3 & -1 & -1 & -1 \\ 3 & 3 & -3 & -3 & -1 & 3 & 1 & 1 \\ 3 & -3 & 3 & -3 & -1 & 1 & 3 & 1 \\ 3 & -3 & -3 & 3 & -1 & 1 & 1 & 3 \end{pmatrix}. \tag{2}$$

The number of linearly independent quartic interactions is given by the rank of $F$. In this case, $\mathrm{rank}(F) = 4$, implying that altogether there are four linearly independent four-fermion terms and the remaining four can be expressed as linearly combinations of the chosen ones. Without the loss of generality, we choose the four singlet interaction terms as the independent ones, and use $F$ to write the quartic terms in the triplet channel as

$$\begin{aligned}
\sum_{s=1}^{3}(\Psi^\dagger\Gamma_{0s}\Psi)^2 &= -2(\Psi^\dagger\Gamma_{00}\Psi)^2 - (\Psi^\dagger\Gamma_{10}\Psi)^2 - (\Psi^\dagger\Gamma_{20}\Psi)^2 - (\Psi^\dagger\Gamma_{30}\Psi)^2, \\
\sum_{s=1}^{3}(\Psi^\dagger\Gamma_{1s}\Psi)^2 &= -(\Psi^\dagger\Gamma_{00}\Psi)^2 - 2(\Psi^\dagger\Gamma_{10}\Psi)^2 + (\Psi^\dagger\Gamma_{20}\Psi)^2 + (\Psi^\dagger\Gamma_{30}\Psi)^2, \\
\sum_{s=1}^{3}(\Psi^\dagger\Gamma_{2s}\Psi)^2 &= -(\Psi^\dagger\Gamma_{00}\Psi)^2 + (\Psi^\dagger\Gamma_{10}\Psi)^2 - 2(\Psi^\dagger\Gamma_{20}\Psi)^2 + (\Psi^\dagger\Gamma_{30}\Psi)^2, \\
\sum_{s=1}^{3}(\Psi^\dagger\Gamma_{3s}\Psi)^2 &= -(\Psi^\dagger\Gamma_{00}\Psi)^2 + (\Psi^\dagger\Gamma_{10}\Psi)^2 + (\Psi^\dagger\Gamma_{20}\Psi)^2 - 2(\Psi^\dagger\Gamma_{30}\Psi)^2.
\end{aligned} \tag{3}$$

In the renormalization group procedure whenever we generate one of these terms, it is always cast back in term of

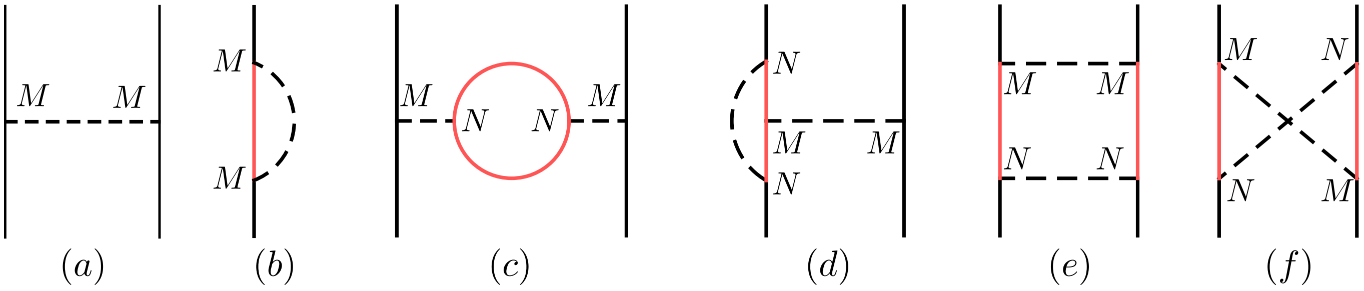


Figure 1. (a) Bare four-fermion interaction vertex $g_M(\Psi^\dagger M \Psi)^2$. (b) The fermionic self-energy correction due to four-fermion interaction, renormalizing the chemical potential $\mu$, and momentum independent (dependent) mass $m$ ($b$). Feynman diagrams (c)–(f) yield corrections to the bare interaction vertex to the leading order in the $\epsilon$ expansion. Here $M$ and $N$ are Hermitian matrices. Solid black (red) lines represent fermionic slow (fast) modes with momentum $|\mathbf{k}| < \Lambda e^{-\ell}$ ($\Lambda e^{-\ell} < |\mathbf{k}| < \Lambda$), where $\Lambda$ is the ultraviolet momentum cutoff and $\ell$ is the logarithm of the renormalization group scale.

the interactions in the singlet channels. This way the interacting action remains closed under coarse grain up to any order in the perturbation theory.

## II. DETAILS OF THE RG FLOW EQUATIONS

In this section, we provide the explicit form of the renormalziation group flow equations of the four independent coupling constants $g^{\rm s}_\beta$, as well as that of the source terms $\Delta^{\rm s}_\beta$, $\Delta^{\rm t}_\beta$, and $\Delta^{\rm p}_\beta$ (see Table I of the main manuscript). After evaluating the Feynman diagrams in Fig. 1, the renormalization group flow equations (also known as the beta functions) of the dimensionless coupling constants (defined in the main manuscript) read

$$
\begin{aligned}
\frac{dg^{\rm s}_0}{d\ell} =& -2g^{\rm s}_0 + (-4f_0 - 14f_k - 2f_\omega + 2\tilde{f}_k - 2\tilde{f}_\omega)(g^{\rm s}_0)^2 + (-2f_k + 2f_\omega + 2\tilde{f}_k - 2\tilde{f}_\omega)(g^{\rm s}_3)^2 + (-2f_k + 2f_\omega + 2\tilde{f}_k - 2\tilde{f}_\omega)(g^{\rm s}_1)^2 + \\
& (-2f_k + 2f_\omega + 2\tilde{f}_k - 2\tilde{f}_\omega)(g^{\rm s}_2)^2 + (8f_0 + 8f_k + 4f_\omega + 4\tilde{f}_0 - 4\tilde{f}_k)g^{\rm s}_0 g^{\rm s}_3 + (4f_0 + 4f_k + 4f_\omega + 8\tilde{f}_k)g^{\rm s}_0 g^{\rm s}_1 + \\
& (4f_0 + 8f_k + 4f_\omega - 4\tilde{f}_k)g^{\rm s}_0 g^{\rm s}_2 + (-4f_k + 4\tilde{f}_k)g^{\rm s}_3 g^{\rm s}_1 + (-8f_k - 8\tilde{f}_k)g^{\rm s}_3 g^{\rm s}_2 + (4f_0 - 4f_k - 4\tilde{f}_0 + 4\tilde{f}_k)g^{\rm s}_1 g^{\rm s}_2, \\
\frac{dg^{\rm s}_1}{d\ell} =& (-4f_k + 4\tilde{f}_k)(g^{\rm s}_0)^2 + (-4f_k + 4\tilde{f}_k)(g^{\rm s}_3)^2 + (4f_0 - 16f_k - 4f_\omega + 4\tilde{f}_k)(g^{\rm s}_1)^2 + (-4f_k + 4\tilde{f}_k)(g^{\rm s}_2)^2 + (4f_k + 4\tilde{f}_k)g^{\rm s}_0 g^{\rm s}_3 + \\
& (-4f_0 + 8f_k + 8f_\omega + 4\tilde{f}_k - 4\tilde{f}_\omega)g^{\rm s}_0 g^{\rm s}_1 + (4f_0 + 4f_k - 4\tilde{f}_0 + 4\tilde{f}_k)g^{\rm s}_0 g^{\rm s}_2 + (8f_0 - 8f_k - 4f_\omega + 4\tilde{f}_0 - 4\tilde{f}_k)g^{\rm s}_3 g^{\rm s}_1 + \\
& (-4f_k + 4f_\omega - 4\tilde{f}_k + 4\tilde{f}_\omega)g^{\rm s}_3 g^{\rm s}_2 + (4f_0 - 8f_k - 4f_\omega - 4\tilde{f}_k)g^{\rm s}_1 g^{\rm s}_2, \\
\frac{dg^{\rm s}_2}{d\ell} =& (2f_k - 2\tilde{f}_k)(g^{\rm s}_0)^2 + (2f_k - 2\tilde{f}_k)(g^{\rm s}_3)^2 + (2f_k - 2\tilde{f}_k)(g^{\rm s}_1)^2 + (4f_0 + 14f_k - 4f_\omega - 2\tilde{f}_k)(g^{\rm s}_2)^2 + (-8f_k - 8\tilde{f}_k)g^{\rm s}_0 g^{\rm s}_3 + \\
& (4f_0 - 4f_k - 4\tilde{f}_0 + 4\tilde{f}_k)g^{\rm s}_0 g^{\rm s}_1 + (-4f_0 - 8f_k + 8f_\omega + 4\tilde{f}_k - 4\tilde{f}_\omega)g^{\rm s}_0 g^{\rm s}_2 + (4f_k + 4f_\omega - 4\tilde{f}_k + 4\tilde{f}_\omega)g^{\rm s}_3 g^{\rm s}_1 + \\
& (8f_0 + 8f_k - 4f_\omega + 4\tilde{f}_0 - 4\tilde{f}_k)g^{\rm s}_3 g^{\rm s}_2 + (4f_0 + 4f_k - 4f_\omega + 8\tilde{f}_k)g^{\rm s}_1 g^{\rm s}_2, \\
\frac{dg^{\rm s}_3}{d\ell} =& (2f_0 + 2f_k + 2\tilde{f}_0 - 2\tilde{f}_k)(g^{\rm s}_0)^2 + (-2f_0 + 14f_k - 4f_\omega + 2\tilde{f}_0 - 2\tilde{f}_k)(g^{\rm s}_3)^2 + (2f_0 + 2f_k + 2\tilde{f}_0 - 2\tilde{f}_k)(g^{\rm s}_1)^2 + \\
& (2f_0 + 2f_k + 2\tilde{f}_0 - 2\tilde{f}_k)(g^{\rm s}_2)^2 + (4f_0 - 8f_k + 8f_\omega + 4\tilde{f}_k - 4\tilde{f}_\omega)g^{\rm s}_0 g^{\rm s}_3 + (-4f_k + 4\tilde{f}_k)g^{\rm s}_0 g^{\rm s}_1 + (-8f_k - 8\tilde{f}_k)g^{\rm s}_0 g^{\rm s}_2 + \\
& (-4f_0 + 4f_k - 4f_\omega + 8\tilde{f}_k)g^{\rm s}_3 g^{\rm s}_1 + (-4f_0 + 8f_k - 4f_\omega - 4\tilde{f}_k)g^{\rm s}_3 g^{\rm s}_2 + (4f_k + 4f_\omega - 4\tilde{f}_k + 4\tilde{f}_\omega)g^{\rm s}_1 g^{\rm s}_2. \\
& .
\end{aligned}
$$

On the other hand, the beta functions of the susceptibilities are obtained by computing the diagrams in Fig. 2, and they are of the form (also expressed in terms of the dimensionless coupling constants)

$$
\begin{aligned}
\frac{d\Delta^{\rm s}_0}{d\ell} &= -2(f_0 + 3f_i + f_\omega)(3g^{\rm s}_0 - g^{\rm s}_3 - g^{\rm s}_1 - g^{\rm s}_2), \\
\frac{d\Delta^{\rm s}_1}{d\ell} &= -2(f_0 - 3f_i - f_\omega)(g^{\rm s}_0 - g^{\rm s}_3 - 3g^{\rm s}_1 - g^{\rm s}_2),
\end{aligned}
$$

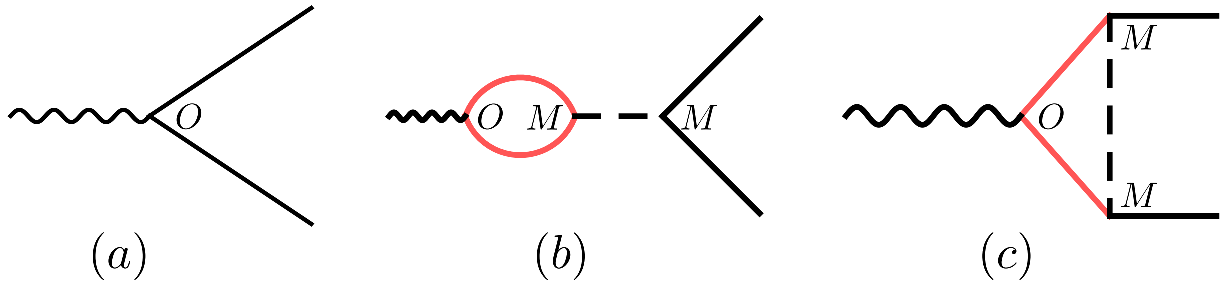


Figure 2. (a) The bare vertex associated with the source term $\Delta_O \Psi^\dagger O \Psi$, where $O$ is a Hermitian matrix. Such vertices are renormalized in the leading order by the Feynman diagrams (b) and (c) due to the quartic interaction of the form $g_M (\Psi^\dagger M \Psi)^2$, yielding the renormalization group flow of the associated conjugate field $\Delta_O$. Here dashed line represents the interaction vertex, while wavy (solid) lines stand for the conjugate field (fermions). The black (red) solid lines represent slow (fast) fermionic modes. See the caption of Fig. 1.

$$
\begin{aligned}
\frac{\mathrm{d}\Delta_2^{\mathrm{s}}}{\mathrm{d}\ell} &= -2(f_0 + 3f_i - f_\omega)(g_0^{\mathrm{s}} - g_3^{\mathrm{s}} - g_1^{\mathrm{s}} - 3g_2^{\mathrm{s}}),\\
\frac{\mathrm{d}\Delta_3^{\mathrm{s}}}{\mathrm{d}\ell} &= 2(f_0 - 3f_i + f_\omega)(g_0^{\mathrm{s}} - 3g_3^{\mathrm{s}} - g_1^{\mathrm{s}} - g_2^{\mathrm{s}}),\\
\frac{\mathrm{d}\Delta_0^{\mathrm{t}}}{\mathrm{d}\ell} &= 2(f_0 - f_i + f_\omega)(g_0^{\mathrm{s}} + g_3^{\mathrm{s}} + g_1^{\mathrm{s}} + g_2^{\mathrm{s}}),\\
\frac{\mathrm{d}\Delta_1^{\mathrm{t}}}{\mathrm{d}\ell} &= -2(f_0 + f_i - f_\omega)(g_0^{\mathrm{s}} - g_3^{\mathrm{s}} + g_1^{\mathrm{s}} - g_2^{\mathrm{s}}),\\
\frac{\mathrm{d}\Delta_2^{\mathrm{t}}}{\mathrm{d}\ell} &= -2(f_0 - f_i - f_\omega)(g_0^{\mathrm{s}} - g_3^{\mathrm{s}} - g_1^{\mathrm{s}} + g_2^{\mathrm{s}}),\\
\frac{\mathrm{d}\Delta_3^{\mathrm{t}}}{\mathrm{d}\ell} &= 2(f_0 + f_i + f_\omega)(g_0^{\mathrm{s}} + g_3^{\mathrm{s}} - g_1^{\mathrm{s}} - g_2^{\mathrm{s}}),\\
\frac{\mathrm{d}\Delta_0^{\mathrm{p}}}{\mathrm{d}\ell} &= 2(\tilde{f}_0 + 3\tilde{f}_k - \tilde{f}_\omega)(g_0^{\mathrm{s}} + g_3^{\mathrm{s}} + g_1^{\mathrm{s}} - g_2^{\mathrm{s}}),\\
\frac{\mathrm{d}\Delta_1^{\mathrm{p}}}{\mathrm{d}\ell} &= -2(\tilde{f}_0 - 3\tilde{f}_k + \tilde{f}_\omega)(g_0^{\mathrm{s}} - g_3^{\mathrm{s}} + g_1^{\mathrm{s}} + g_2^{\mathrm{s}}),\\
\frac{\mathrm{d}\Delta_2^{\mathrm{p}}}{\mathrm{d}\ell} &= -2(\tilde{f}_0 - \tilde{f}_k + \tilde{f}_\omega)(g_0^{\mathrm{s}} - g_3^{\mathrm{s}} - g_1^{\mathrm{s}} - g_2^{\mathrm{s}}),\\
\frac{\mathrm{d}\Delta_3^{\mathrm{p}}}{\mathrm{d}\ell} &= 2(\tilde{f}_0 - 3\tilde{f}_k - \tilde{f}_\omega)(g_0^{\mathrm{s}} + g_3^{\mathrm{s}} - g_1^{\mathrm{s}} + g_2^{\mathrm{s}}).
\end{aligned}
$$

The functions appearing in the renormalization group flow equations are functions of dimensionless temperature $t$ and chemical potential $\mu$, as well as the dimensionless masses $m$ and $b$, defined in the main manuscript. They are derived from the loop integrals and given by

$$
\begin{aligned}
I_\omega &= T\sum_{\omega_n}\int' \frac{\mathrm{d}\mathbf{k}}{(2\pi)^d}\frac{\Omega_+^2}{(\Omega_+^2 - \epsilon_{\mathbf{k}}^2)^2} = -\frac{1}{2\pi^2}\frac{\Lambda^d}{v\Lambda} f_\omega(t,\mu,m,b)\ell,\\
\tilde{I}_\omega &= T\sum_{\omega_n}\int' \frac{\mathrm{d}\mathbf{k}}{(2\pi)^d}\frac{\Omega_+\Omega_-}{(\Omega_+^2 - \epsilon_{\mathbf{k}}^2)(\Omega_-^2 - \epsilon_{\mathbf{k}}^2)} = -\frac{1}{2\pi^2}\frac{\Lambda^d}{v\Lambda} \tilde{f}_\omega(t,\mu,m,b)\ell,\\
I_0 &= T\sum_{\omega_n}\int' \frac{\mathrm{d}\mathbf{k}}{(2\pi)^d}\frac{(m+bk^2)^2}{(\Omega_+^2 - \epsilon_{\mathbf{k}}^2)^2} = \frac{1}{2\pi^2}\frac{\Lambda^d}{v\Lambda} f_0(t,\mu,m,b)\ell,\\
\tilde{I}_0 &= T\sum_{\omega_n}\int' \frac{\mathrm{d}\mathbf{k}}{(2\pi)^d}\frac{(m+bk^2)^2}{(\Omega_+^2 - \epsilon_{\mathbf{k}}^2)(\Omega_-^2 - \epsilon_{\mathbf{k}}^2)} = \frac{1}{2\pi^2}\frac{\Lambda^d}{v\Lambda} \tilde{f}_0(t,\mu,m,b)\ell,\\
I_k &= T\sum_{\omega_n}\int' \frac{\mathrm{d}\mathbf{k}}{(2\pi)^d}\frac{v^2 k_i^2}{(\Omega_+^2 - \epsilon_{\mathbf{k}}^2)^2} = \frac{1}{2\pi^2}\frac{\Lambda^d}{v\Lambda} f_k(t,\mu,m,b)\ell,
\end{aligned}
$$

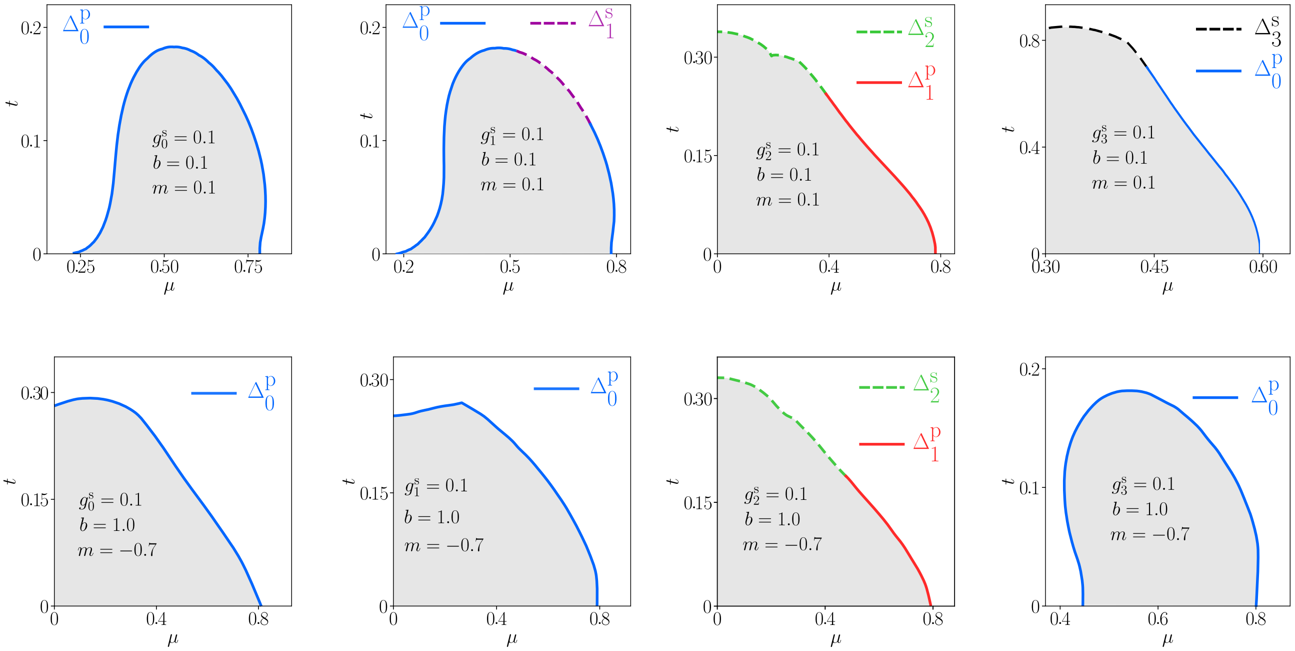


Figure 3. Phase diagrams in the $(\mu, t)$ plane with interactions in individual singlet channels for fixed (positive) $g^{\rm s}_\beta > 0$. Here $\beta = 0, 1, 2,$and 3 in the first, second, third, and fourth columns, respectively, and the top (bottom) row corresponds to the trivial (topological) insulating phase in the normal state when $\mu = 0$. The bare values of $g^{\rm s}_\beta$, $b$, and $m$ are quoted in each panel. The white region corresponds to Fermi liquid, while the ordered phase is shown in gray. At the phase boundary the leading instability is shown (color coded), where the solid (dashed) line marks superconducting (excitonic) ordering.

with the explicit functional forms

$$f_\omega(t,\mu,m,b) = \sum_{\tau=\pm}\left(\frac{\text{sech}^2\left(\frac{E_\Lambda+\tau\mu}{2t}\right)}{16t} + \frac{\tanh\left(\frac{E_\Lambda+\tau\mu}{2t}\right)}{8E_\Lambda}\right),$$

$$\tilde{f}_\omega(t,\mu,m,b) = \sum_{\tau=\pm}\frac{\tau\tanh(\frac{E_\Lambda+\tau\mu}{2t})(E_\Lambda^2+\tau E_\Lambda\mu-2\mu^2)}{8\mu(E_\Lambda^2-\mu^2)},$$

$$f_0(t,\mu,m,b) = (m+b)^2\sum_{\tau=\pm}\left(-\frac{\text{sech}^2\left(\frac{E_\Lambda+\tau\mu}{2t}\right)}{16E_\Lambda^2 t} + \frac{\tanh\left(\frac{E_\Lambda+\tau\mu}{2t}\right)}{8E_\Lambda^3}\right),$$

$$\tilde{f}_0(t,\mu,m,b) = (m+b)^2\sum_{\tau=\pm}\frac{\tau\tanh(\frac{E_\Lambda-\tau\mu}{2t})(E_\Lambda-\tau\mu)}{8E_\Lambda\mu(E_\Lambda^2-\mu^2)},$$

$$f_k(t,\mu,m,b) = \sum_{\tau=\pm}\left(-\frac{\text{sech}^2\left(\frac{E_\Lambda+\tau\mu}{2t}\right)}{16E_\Lambda^2 t} + \frac{\tanh\left(\frac{E_\Lambda+\tau\mu}{2t}\right)}{8E_\Lambda^3}\right),$$

$$\tilde{f}_k(t,\mu,m,b) = \sum_{\tau=\pm}\frac{\tau\tanh(\frac{E_\Lambda-\tau\mu}{2t})(E_\Lambda-\tau\mu)}{8E_\Lambda\mu(E_\Lambda^2-\mu^2)},$$

where $E_\Lambda = \sqrt{1/2+(m+b)^2}$. Here $\omega_n = (2n+1)\pi T$ is the fermionic Matsubara frequency with $-\infty \le n \le \infty$ as integer, $\Omega_\pm = i\omega_n \pm \mu$, and the prime symbol in the momentum integral indicates that the corresponding radial integration is restricted within the thin Wilsonian momentum shell $\Lambda e^{-\ell} < |\mathbf{k}| < \Lambda$. Here, $\Lambda$ is the ultraviolet momentum cutoff and $\ell$ is the logarithm of the renormalization group scale.

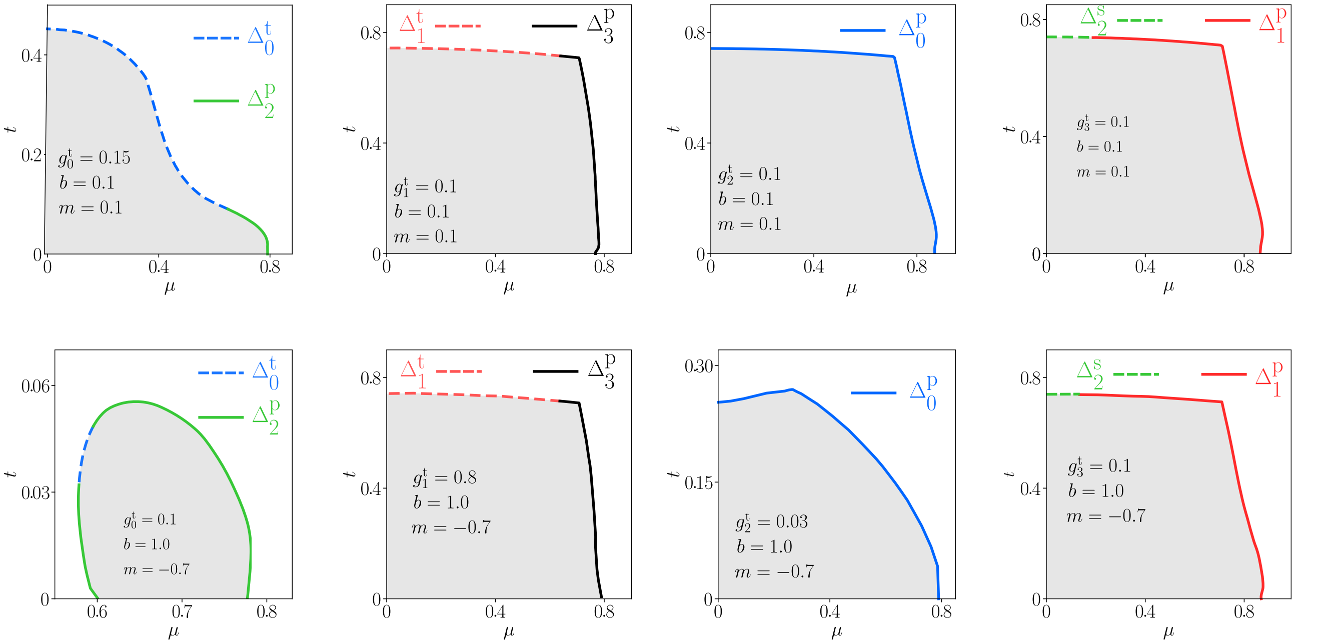

Figure 4. Phase diagrams in the $(\mu, t)$ plane with interactions in individual channels for fixed (positive) $g^{\rm t}_\beta > 0$. Here $\mu = 0, 1, 2,$ and 3 in the first, second, third, and fourth columns, respectively, and the top (bottom) row corresponds to the trivial (topological) insulator in the normal state when $\mu = 0$. The bare values of $g^{\rm t}_\mu$, $b$, and $m$ are shown in each panel. The rest of the notations and symbols are the same as in Fig. 3.

## III. PHASE DIAGRAMS FOR INDIVIDUAL INTERACTION CHANNELS

In this section, we display the phase diagram in the $(\mu, t)$ plane for individual repulsive interactions $g^\alpha_\beta > 0$ for a given $\beta = 0, 1, 2, 3$ and $\alpha$ = s and t for the singlet and triplet channels, respectively, and all other coupling constants set to zero. The resulting excitonic and pairing orders for various interaction channels are summarized in Table II of the main text, and their correspondence substantiates the selection rules outlined also in the main text and Table II. The phase diagrams for singlet and triplet channels are shown in Fig. 3, and Fig. 4, respectively. Besides the selection rule between a given interaction channel and the resulting ordered phase(s), we also notice a generic feature of all these phase diagrams. While the ordered states are realized in the low temperature regime, causing gain in the condensation energy, the high temperature phase is the Fermi liquid, harboring gapless quasiparticles without any symmetry breaking, with maximal entropy. This observation is consistent with the recently proposed 'organization principle' from Refs. [2, 3].

[1] I. F. Herbut, V. Juričić, and B. Roy, Phys. Rev. B **79**, 085116 (2009).
[2] A. L. Szabó, R. Moessner, and B. Roy, Phys. Rev. B **103**, 165139 (2021).
[3] A. L. Szabó and B. Roy, Phys. Rev. B **103**, 205135 (2021).
